# Supplementary material for: Abstract Transducers
Source: arXiv:1910.07583 source file (2019-10-16)
Supplement: Supplementary file 1 [file appendix.tex]

\section{Implementation}

\begin{figure}[tp]
\begin{subfigure}[b]{.49\linewidth}
\centering
\begin{tikzpicture}[node distance=12mm, scale=0.7, transform shape,auto]
\node[] at (0.5,0.5) (top) {};
\node[] at (0.5,-8) (bottom) {};

\node[] (qs) {};
\node[] at (0,-8) (ql) {$~$};
\node[cfastate,below of=qs,minimum size=8mm] (q1) {$q_1$};
\node[cfastate,below=of q1,minimum size=8mm] (q2) {$q_2$};
\node[cfatargetstate,below=of q2,minimum size=8mm] (q3) {$q_3$};
\node[cfatargetstate,below=of q3,minimum size=8mm] (q4) {$q_4$};

\path[trans,two] (q1) edge [loop left] node [anchor=center,left] {\textsf{else}} (q1);
\path[trans,two] (q2) edge [loop right] node [anchor=center,right] {\textsf{else}} (q2);

\path[trans] (qs) edge [] node [anchor=center,above] {} (q1);

\path[trans,two] (q1) edge [bend right] node [anchor=center,right] {$a$} (q2);
\path[trans,two] (q2) edge [] node [anchor=center,left] {$a$} (q3);
\path[trans,two] (q2) edge [bend right] node [anchor=center,right] {$b$} (q1);
\path[trans,two] (q1) edge [bend right] node [anchor=center,left] {$b$} (q4);
\end{tikzpicture}
\begin{tikzpicture}[node distance=12mm, scale=0.7, transform shape,auto]
\node[] at (0.7,0.5) (top) {};
\node[] at (0.7,-8) (bottom) {};

\node[] (qs) {};
\node[] at (0,-8) (ql) {$~$};
\node[cfastate,below of=qs,minimum size=8mm] (q1) {$q_5$};
\node[cfastate,below=of q1,minimum size=8mm] (q2) {$q_6$};
\node[cfatargetstate,below=of q2,minimum size=8mm] (q3) {$q_7$};
\node[cfatargetstate,below=of q3,minimum size=8mm] (q4) {$q_8$};

\path[trans,one] (q1) edge [loop left] node [anchor=center,left] {\textsf{else}} (q1);
\path[trans,one] (q2) edge [loop right] node [anchor=center,right] {\textsf{else}} (q2);

\path[trans] (qs) edge [] node [anchor=center,above] {} (q1);

\path[trans,one] (q1) edge [bend right] node [anchor=center,right] {$c$} (q2);
\path[trans,one] (q2) edge [] node [anchor=center,left] {$c$} (q3);
\path[trans,one] (q2) edge [bend right] node [anchor=center,right] {$d$} (q1);
\path[trans,one] (q1) edge [bend right] node [anchor=center,left] {$d$} (q4);
\end{tikzpicture}
\caption{}
\end{subfigure}
\begin{subfigure}[b]{.49\linewidth}
\centering
\begin{tikzpicture}[node distance=12mm, scale=0.7, transform shape,auto]

\node[] at (1.8,0.5) (top) {};
\node[] at (1.8,-9) (bottom) {};

\node[] (qs) {};
\node[] at (0,-9) (ql) {$~$};
\node[cfastate,below of=qs,minimum size=8mm] (q0) {$q_0$};

\path[trans] (qs) edge [] node [anchor=center,above] {} (q0);

\node[cfastate,minimum size=8mm] at (-1.4,-2) (q1) {$q_1$};
\node[cfastate,below=of q1,minimum size=8mm] (q2) {$q_2$};
\node[cfatargetstate,below=of q2,minimum size=8mm] (q3) {$q_3$};
\node[cfatargetstate,below=of q3,minimum size=8mm] (q4) {$q_4$};

\node[cfastate,minimum size=8mm] at (1.4,-2) (q5) {$q_5$};
\node[cfastate,below=of q5,minimum size=8mm] (q6) {$q_6$};
\node[cfatargetstate,below=of q6,minimum size=8mm] (q7) {$q_7$};
\node[cfatargetstate,below=of q7,minimum size=8mm] (q8) {$q_8$};

\path[trans,two] (q1) edge [loop left] node [anchor=center,left] {\textsf{else}} (q1);
\path[trans,two] (q2) edge [loop right] node [anchor=center,right] {\textsf{else}} (q2);

\path[trans,one] (q5) edge [loop left] node [anchor=center,left] {\textsf{else}} (q5);
\path[trans,one] (q6) edge [loop right] node [anchor=center,right] {\textsf{else}} (q6);

\path[trans,two] (q1) edge [bend right] node [anchor=center,right] {$a$} (q2);
\path[trans,two] (q2) edge [] node [anchor=center,left] {$a$} (q3);
\path[trans,two] (q2) edge [bend right] node [anchor=center,right] {$b$} (q1);
\path[trans,two] (q1) edge [bend right] node [anchor=center,left] {$b$} (q4);

\path[trans,one] (q5) edge [bend right] node [anchor=center,right] {$c$} (q6);
\path[trans,one] (q6) edge [] node [anchor=center,left] {$c$} (q7);
\path[trans,one] (q6) edge [bend right] node [anchor=center,right] {$d$} (q5);
\path[trans,one] (q5) edge [bend right] node [anchor=center,left] {$d$} (q8);

\path[trans] (q0) edge [bend right] node [anchor=center,above] {$\epsilon$} (q1);
\path[trans] (q0) edge [bend left] node [anchor=center,above] {$\epsilon$} (q5);
\end{tikzpicture}
\caption{}
\end{subfigure}

\begin{subfigure}[b]{.49\linewidth}
\centering
\begin{tikzpicture}[node distance=12mm, scale=0.7, transform shape,auto]

\node[] at (1.8,0.5) (top) {};
\node[] at (1.8,-9) (bottom) {};

\node[] (qs) {};
\node[] at (0,-9) (ql) {$~$};
\node[cfastate,below of=qs,minimum size=8mm] (q0) {$q_0$};

\path[trans] (qs) edge [] node [anchor=center,above] {} (q0);

\node[cfatargetstate,minimum size=8mm] at (-2,-2) (q4) {$q_4$};
\node[cfastate,below=of q4,minimum size=8mm] (q1) {$q_1$};
\node[cfastate,minimum size=8mm] at (-1.5,-6) (q2) {$q_2$};
\node[cfatargetstate,below=of q2,minimum size=8mm] (q3) {$q_3$};

\node[cfatargetstate,minimum size=8mm] at (2,-2) (q8) {$q_8$};
\node[cfastate,below=of q8,minimum size=8mm] (q5) {$q_5$};
\node[cfastate,minimum size=8mm] at (1.5,-6) (q6) {$q_6$};
\node[cfatargetstate,below=of q6,minimum size=8mm] (q7) {$q_7$};

\path[trans,two] (q1) edge [loop left] node [anchor=center,left] {$\lnot (a \lor b)$} (q1);
\path[trans,two] (q2) edge [loop left] node [anchor=center,left] {$\lnot (a \lor b)$} (q2);

\path[trans,one] (q5) edge [loop right] node [anchor=center,right] {$\lnot (c \lor d)$} (q5);
\path[trans,one] (q6) edge [loop right] node [anchor=center,right] {$\lnot (c \lor d)$} (q6);

\path[trans,two] (q0) edge [sloped] node [anchor=center,above] {$\lnot (a \lor b)$} (q1);
\path[trans,one] (q0) edge [sloped] node [anchor=center,above] {$\lnot (c \lor d)$} (q5);

\path[trans,two] (q1) edge [bend right] node [anchor=center,left] {$a$} (q2);
\path[trans,two] (q2) edge [] node [anchor=center,left] {$a$} (q3);
\path[trans,two] (q2) edge [bend right] node [anchor=center,left] {$b$} (q1);
\path[trans,two] (q1) edge [] node [anchor=center,left] {$b$} (q4);

\path[trans,one] (q5) edge [bend right] node [anchor=center,right] {$c$} (q6);
\path[trans,one] (q6) edge [] node [anchor=center,right] {$c$} (q7);
\path[trans,one] (q6) edge [bend right] node [anchor=center,right] {$d$} (q5);
\path[trans,one] (q5) edge [] node [anchor=center,right] {$d$} (q8);

\path[trans,two] (q0) edge [] node [anchor=center,above] {$b$} (q4);
\path[trans,one] (q0) edge [] node [anchor=center,above] {$d$} (q8);

\path[trans,two] (q0) edge [] node [anchor=center,left] {$a$} (q2);
\path[trans,one] (q0) edge [] node [anchor=center,right] {$c$} (q6);
\end{tikzpicture}
\caption{}
\end{subfigure}
\begin{subfigure}[b]{.49\linewidth}
\centering
\begin{tikzpicture}[node distance=12mm, scale=0.7, transform shape,auto]
\node[] (qs) {};

\node[cfastate,below=of qs] (q15) {$q_{1|5}$};
\node[cfastate,right=of q15] (q16) {$q_{1|6}$};
\node[cfatargetstate,right=of q16] (q17) {$q_{1|7}$};
\node[cfatargetstate,right=of q17] (q18) {$q_{1|8}$};

\node[cfastate,below=of q15]  (q25) {$q_{2|5}$};
\node[cfastate,right=of q25] (q26) {$q_{2|6}$};
\node[cfatargetstate,right=of q26] (q27) {$q_{2|7}$};
\node[cfatargetstate,right=of q27] (q28) {$q_{2|8}$};

\node[cfatargetstate,below=of q25]  (q35) {$q_{3|5}$};
\node[cfatargetstate,right=of q35] (q36) {$q_{3|6}$};
\node[cfatargetstate,right=of q36] (q37) {$q_{3|7}$};
\node[cfatargetstate,right=of q37] (q38) {$q_{3|8}$};

\node[cfatargetstate,below=of q35]  (q45) {$q_{4|5}$};
\node[cfatargetstate,right=of q45] (q46) {$q_{4|6}$};
\node[cfatargetstate,right=of q46] (q47) {$q_{4|7}$};
\node[cfatargetstate,right=of q47] (q48) {$q_{4|8}$};

\path[trans] (qs) edge [] node [anchor=center,above] {} (q15);

\path[trans,two] (q15) edge [bend right] node [anchor=center,left] {$a$} (q25);
\path[trans,two] (q16) edge [bend right] node [anchor=center,left] {$a$} (q26);
\path[trans,two] (q17) edge [bend right] node [anchor=center,left] {$a$} (q27);
\path[trans,two] (q18) edge [bend right] node [anchor=center,left] {$a$} (q28);

\path[trans,two] (q15) edge [bend right] node [anchor=center,left] {$b$} (q45);
\path[trans,two] (q16) edge [bend right] node [anchor=center,left] {$b$} (q46);
\path[trans,two] (q17) edge [bend right] node [anchor=center,left] {$b$} (q47);
\path[trans,two] (q18) edge [bend right] node [anchor=center,left] {$b$} (q48);

\path[trans,two] (q25) edge [bend right] node [anchor=center,left] {$b$} (q15);
\path[trans,two] (q26) edge [bend right] node [anchor=center,left] {$b$} (q16);
\path[trans,two] (q27) edge [bend right] node [anchor=center,left] {$b$} (q17);
\path[trans,two] (q28) edge [bend right] node [anchor=center,left] {$b$} (q18);

\path[trans,two] (q25) edge [] node [anchor=center,left] {$a$} (q35);
\path[trans,two] (q26) edge [] node [anchor=center,left] {$a$} (q36);
\path[trans,two] (q27) edge [] node [anchor=center,left] {$a$} (q37);
\path[trans,two] (q28) edge [] node [anchor=center,left] {$a$} (q38);

\path[trans,one] (q15) edge [bend right] node [anchor=center,above] {$c$} (q16);
\path[trans,one] (q25) edge [bend right] node [anchor=center,above] {$c$} (q26);
\path[trans,one] (q35) edge [bend right] node [anchor=center,above] {$c$} (q36);
\path[trans,one] (q45) edge [bend right] node [anchor=center,above] {$c$} (q46);

\path[trans,one] (q16) edge [] node [anchor=center,above] {$c$} (q17);
\path[trans,one] (q26) edge [] node [anchor=center,above] {$c$} (q27);
\path[trans,one] (q36) edge [] node [anchor=center,above] {$c$} (q37);
\path[trans,one] (q46) edge [] node [anchor=center,above] {$c$} (q47);

\path[trans,one] (q16) edge [bend right] node [anchor=center,above] {$d$} (q15);
\path[trans,one] (q26) edge [bend right] node [anchor=center,above] {$d$} (q25);
\path[trans,one] (q36) edge [bend right] node [anchor=center,above] {$d$} (q35);
\path[trans,one] (q46) edge [bend right] node [anchor=center,above] {$d$} (q45);

\path[trans,one] (q15) edge [bend right] node [anchor=center,above] {$d$} (q18);
\path[trans,one] (q25) edge [bend right] node [anchor=center,above] {$d$} (q28);
\path[trans,one] (q35) edge [bend right] node [anchor=center,above] {$d$} (q38);
\path[trans,one] (q45) edge [bend right] node [anchor=center,above] {$d$} (q48);
\end{tikzpicture}
\caption{}
\end{subfigure}
\caption{Example to illustrate an union of two automata~(a)---for 
transducers, also the output has to be considered.
One approach~\cite{Sipser} is to take advantage of $\epsilon$--transitions, 
which results in the non-deterministic automaton~(b).
The $\epsilon$--transitions can get removed, which results in 
the non-deterministic automaton~(c).
An alternative is to explicitly construct the deterministic 
product automaton~(d), based on a powerset (or subset) construction, 
which can have an exponential number of states.
Please note: That we have \emph{not drawn the stuttering self transitions}
that are present for each of the control states in automaton~(d).}
\label{fig:automata:union}
\end{figure}

We employ the formalism of configurable program analysis to provide the procedure
of computing an abstract epsilon closure and summarize the functionality
in the operator~$\outclosure$:

The operator~$\outclosure: \transducers \times (\atmtstates \times \artefacts) \rightarrow 2^{ \atmtstates \times \artefacts }$ takes as argument a transducer~$\transducer$, one of the transducers control states, 
and an initial abstract artefact, and returns an abstract epsilon closure of state~$q$.
The operator is implicitly parameterized with an \emph{artefact closure 
analysis}, which is a configurable program analysis~$\closureanalysis = (\abstdomain_\artefacts, 
\transabs{}{}_\closureanalysis, \mergeop_\closureanalysis, \stopop_\closureanalysis)$ 
that uses a task artifact domain~$\abstdomain_\artefacts$, that is, it each of its abstract states 
represents an abstract task artefact~$\artefact \in \artefacts$. 
The result of the operator is a map~$\subseteq \atmtstates \times \artefacts$ of 
closure termination states to abstract task artefacts.

% $\closureanalysis = (\lattice, \closurestate_0, \transabs{}{})$

% $\outclosure: \atmtstates \times \controlflows \rightarrow 2^{\atmtstates \times \closurestates}$

% $\closureanalysis = (\artefactdomain, \transabs{}{}, \mergeop, \stopop)$

The artifact closure analysis~$\closureanalysis$ gets composed with an 
analysis~$\transepscpa = (\abstdomain_\epsilon, \transabs{}{}_\epsilon, 
\mergesepop_{\abstdomain_\epsilon}, \stopsepop_{\abstdomain_\epsilon})$ 
that keeps track of the position in the abstract transducer.
This analysis uses a flat-lattice domain~$\abstdomain_\epsilon$ where one abstract 
state corresponds to the control state of the transducer the analysis is conducted on.
Given a task abstract transducer~$\transducer = (\atmtstates, \atmtalgebra, \outalphabet, \atmtfinal, \qinit, \qoff, \atmtrelation, \concernmap) \in \transducers$, 
the transition relation~$\transabs{}{}_\epsilon$
has the transfer~$q \transabs{\transtrans}{}_\epsilon q'$, 
for~$\transtrans = (q, \sigma, q', \cdot) \in \atmtrelation$, if and only if $\sigma = \epsilon$.
